# Supplementary material for: Temporal Poisson Square Root Graphical Models
Source: arXiv:2005.06462 source file (2020-05-12)
Supplement: Supplementary file 1 [file supp.tex]

\appendix
\section{Appendix}

\subsection{Auxiliary Results}
\begin{lemma}
Let $\mathbb{X}$ and $\lambda \in (0,\lambda_{\max}]$ be given. Let $\hat{\btheta}$ be the corresponding primal solution defined in (\ref{eq:interScreen}). Then, by the optimality conditions of (\ref{eq:interScreen}):
\begin{equation}
\label{eq:primal-kkt}
\hat{w}_k := \frac{ \exp \left(- \hat{\theta}_{ii} x_i^{(k)} - \sum_{j \in \tilde{V}} \hat{\theta}_{ij}  \tilde{x}_{j}^{(k)} \right) }{\sum_{k'=1}^n \exp \left(- \hat{\theta}_{ii} x_i^{(k')} - \sum_{j \in \tilde{V}} \hat{\theta}_{ij} \tilde{x}_{j}^{(k')} \right)},\quad - \sum_{k=1}^n \hat{w}_k x_{i}^{(k)} = 0, \quad - \sum_{k=1}^n \hat{w}_k \tilde{x}_{j}^{(k)} + \lambda \hat{t}_j = 0,
\end{equation}
where $\hat{t}_j$ is the $j^{th}$ component of the subgradient of $\hat{\bm{t}} \in \partial \left(\sum_{j \in \tilde{V}} \left\lvert \hat{\theta}_{ij} \right\rvert\right)$.
\end{lemma}

\begin{lemma}
\label{lemma:lambda-max}
Let $\mathbb{X}$ be given. Let $\lambda_{\max}$ be the smallest regularization parameter such that the optimal solution to (\ref{eq:interScreen}) $\hat{\btheta}$ satisfying
$\hat{\btheta}_{\backslash i} := \begin{bmatrix}
\hat{\theta}_{i1} & \cdots & \hat{\theta}_{i(i-1)} & \hat{\theta}_{i (i+1)} & \cdots & \hat{\theta}_{ip}
\end{bmatrix}^\top = \bzero$. Then:
\begin{equation*}
\hat{\theta}_{ii} =  \frac{1}{2} \log \frac{ \lvert \mathcal{P}_i \rvert}{ \lvert \mathcal{N}_i \rvert},\quad \lambda_{\max} = \max_{j\in \tilde{V}} \left\lvert \frac{1}{2 \lvert \mathcal{P}_i \rvert}\sum_{k\in \mathcal{P}_i} x_j^{(k)} - \frac{1}{2 \lvert \mathcal{N}_i \rvert}\sum_{k\in \mathcal{N}_i} x_j^{(k)} \right\rvert \le 1,
\end{equation*}
where $\mathcal{P}_i := \curly{k \mid x_i^{(k)} = 1, k \in \curly{1,2,\cdots,n}}$ and  $\mathcal{N}_i := \curly{k \mid x_i^{(k)} = -1, k \in \curly{1,2,\cdots,n}}$. $\lvert \mathcal{P}_i \rvert$ and $\lvert  \mathcal{N}_i \rvert$ represent the cardinality of $\mathcal{P}_i$ and $\mathcal{N}_i$, respectively.
\end{lemma}

\begin{lemma}
\label{lemma:strong-cvx}
Let $g(\balpha) := \frac{1}{n}\sum_{k=1}^n \alpha_k \log \alpha_k$ be the objective in (\ref{eq:dual}). Let $\mathcal{B} := \curly{\balpha \mid 0<\alpha_k<1,\forall k\in \curly{1,2,\cdots,n}}$. Then $\forall \balpha, \tilde{\balpha} \in \mathcal{B}$,
\begin{equation}
\label{eq:grad-hessian}
\nabla g(\balpha) = \begin{bmatrix}
\frac{1}{n}(\log \alpha_1+1) & \frac{1}{n}(\log \alpha_2+1) & \cdots &\frac{1}{n}(\log \alpha_n+1) \end{bmatrix}^\top,\quad 
\nabla^2g (\balpha) = \mathrm{diag} \left(\frac{1}{n \alpha_1},\frac{1}{n \alpha_2},\cdots,\frac{1}{n \alpha_n}\right),
\end{equation}
where $\nabla g(\balpha)$ is the gradient, $\nabla^2 g(\balpha)$ is the hessian, and $\mathrm{diag}(\cdot)$ represents a diagonal matrix. Furthermore, $\forall \balpha, \tilde{\balpha} \in \mathcal{B}$,
\begin{equation}
\label{eq:ball}
g(\tilde{\balpha}) - g(\balpha) \ge \nabla^\top g(\balpha) (\tilde{\balpha}-\balpha) + \frac{1}{2n} \norm{\tilde{\balpha}-\balpha}_2^2.
\end{equation}
\end{lemma}

\begin{lemma}
\label{lemma:strong-dual}
Let $\mathbb{X}$ and $\lambda \in (0,\lambda_{\max}]$ be given. Then strong duality [] holds between the primal problem (\ref{eq:interScreen}) and the dual problem (\ref{eq:dual}). Furthermore, let $\hat{\balpha}(\lambda_{\max})$ be the dual optimal solution when $\lambda = \lambda_{\max}$, then
\begin{equation*}
\hat{\alpha}_k(\lambda_{\max})  = \begin{cases}
\frac{\sqrt{\lvert \mathcal{P}_i \rvert \lvert \mathcal{N}_i \rvert}}{2\lvert \mathcal{P}_i \rvert^2} & \forall k \in \mathcal{P}_i,\\
\frac{\sqrt{\lvert \mathcal{P}_i \rvert \lvert \mathcal{N}_i \rvert}}{2\lvert \mathcal{N}_i \rvert^2} & \forall k \in \mathcal{N}_i.
\end{cases}
\end{equation*}
Finally, the dual problem (\ref{eq:dual}) is feasible \charles{not proven yet}.
\end{lemma}

\begin{lemma}
\label{lemma:dual-kkt}
Let $\hat{\balpha}$ be the optimal solution to (\ref{eq:dual}), then $\exists \gamma_j^+$,$\gamma_j^->0$, $\forall j \in \tilde{V}$, $\kappa_1$, $\kappa_2 \in \mathbb{R}$, s.t.
\begin{equation*}
\nabla g \left(\hat{\balpha}\right) + \sum_{j \in \tilde{V}} \gamma^+_j \tilde{\bx}_j - \sum_{j \in \tilde{V}} \gamma^-_j \tilde{\bx}_j + \kappa_1 \bx_i + \kappa_2 \bone = \bzero,
\end{equation*}
where $\bx_i = \begin{bmatrix} x_i^{(1)} & x_i^{(2)} & \cdots & x_i^{(n)} \end{bmatrix}^\top$, and $\bone$ is an $n\times 1$ vector of all ones.
\end{lemma}

\begin{lemma} \charles{not proven yet.}
\label{lemma:ball} Let $\lambda_0$ and $\lambda$ be given, where $\lambda_{\max} \ge \lambda_0 > \lambda > 0$. Let $\hat{\balpha}(\lambda_0)$ and $\hat{\balpha}(\lambda)$ be the dual optimal solutions to (\ref{eq:dual}) for $\lambda_0$ and $\lambda$ respectively. Then
\begin{equation}
\label{eq:ball}
r:= \sqrt{2n \left[g\left(\frac{\lambda}{\lambda_0} \hat{\balpha}(\lambda_0)\right) - g(\hat{\balpha}(\lambda_0)) + \left(1-\frac{\lambda}{\lambda_0}\right) \nabla^\top g(\hat{\balpha}(\lambda_0)) \hat{\balpha}(\lambda_0)\right]},\quad \norm{\hat{\balpha}(\lambda)-\hat{\balpha}(\lambda_0)}_2^2 \le r^2.
\end{equation}
\end{lemma}

\subsection{Proof of Lemma~\ref{lemma:dual}}
\label{sec:proof-lemma-dual}
We first introduce the slack variables $q_k$'s, such that
\begin{equation*}
\log q_k = - \theta_{ii} x_i^{(k)}  - \sum_{j \in \tilde{V}} \theta_{ij} \tilde{x}_{j}^{(k)},\quad  \forall k \in \curly{1,2,\cdots,n}.
\end{equation*}
Then the (primal) interaction screening problem (\ref{eq:interScreen}) becomes:
\begin{equation}
\label{eq:interScreen-eq}
\arg\min_{\btheta} \log \left[\frac{1}{n}\sum_{k=1}^n q_k  \right] + \lambda \sum_{j \in \tilde{V}} \lvert \theta_{ij} \rvert,\quad 
\text{s.t. } \log q_k = - \theta_{ii} x_i^{(k)}  - \sum_{j \in \tilde{V}} \theta_{ij} \tilde{x}_{j}^{(k)},\quad \forall k \in \curly{1,2,\cdots,n}.
\end{equation}
The Lagrangian is:
\begin{equation*}
L(\bq, \btheta; \balpha) := \log\left[ \frac{1}{n}\sum_{k=1}^n q_k \right] + \lambda \sum_{j \in \tilde{V}} \lvert \theta_{ij} \rvert + \sum_{k=1}^n \alpha_k \left[- \theta_{ii} x_i^{(k)} - \sum_{j \in \tilde{V}} \theta_{ij} \tilde{x}_{j}^{(k)} - \log q_k \right],
\end{equation*}
where $\bq = \begin{bmatrix} q_1 & q_2 & \cdots & q_n \end{bmatrix}^\top$, $\btheta = \begin{bmatrix}
\theta_{i1} & \theta_{i2} & \cdots & \theta_{ip}
\end{bmatrix}^\top$, and $\balpha = \begin{bmatrix} \alpha_1 & \alpha_2 & \cdots & \alpha_n \end{bmatrix}^\top$. In order to formulate the dual problem, we first need to solve the following optimization problems with respect to the primal parameters $\bq$ and $\btheta$:
\begin{align}
\label{eq:L1}
\bq^\dag := \arg\min_{\bq} L_1(\bq) := & \arg\min_\bq \log\left[ \frac{1}{n}\sum_{k=1}^n q_k \right] - \sum_{k=1}^n \alpha_k \log q_k;\\
\label{eq:L2}
\btheta^\dag := \arg\min_{\btheta} L_2 \left(\btheta\right) := & \arg\min_{\btheta} \theta_{ii} \left(-\sum_{k=1}^n \alpha_k x_i^{(k)}\right) + \lambda \sum_{j \in \tilde{V}} \lvert \theta_{ij} \rvert - \frac{1}{n} \sum_{k=1}^n   \sum_{j \in \tilde{V}} \theta_{ij} \alpha_k  \tilde{x}_{j}^{(k)}.
\end{align}

\begin{itemize}[leftmargin=*]
\item To solve (\ref{eq:L1}), by KKT conditions,
\begin{equation}
\label{eq:kkt-q}
\frac{\partial L_1(\bq^\dag) }{\partial q_k^\dag} =  \frac{1}{\sum_{k'=1}^n q_{k'}^\dag} - \frac{\alpha_k}{q_k^\dag} = 0 \Rightarrow \frac{q_k^\dag}{\sum_{k'=1}^n q_{k'}^\dag} = \alpha_k \Rightarrow \sum_{k=1}^n \alpha_k = 1.
\end{equation}
Furthermore since $q_k^\dag >0$, $\forall k \in \curly{1,2,\cdots,n}$, we have
\begin{equation}
\label{eq:kkt-q-2}
0 < \alpha_k < 1,\quad \forall k \in \curly{1,2,\cdots,n}.
\end{equation}

Let $C = \sum_{k=1}^n q_{k}^\dag$. Let $\bq=\bq^\dag$ in $L_1(\bq)$.  We have that
\begin{align}
\label{eq:kkt-q-3}
\begin{split}
\min_\bq L_1(\bq) = & L_1(\bq^\dag) = \log\left[ \frac{1}{n}\sum_{k=1}^n q_k^\dag \right] - \sum_{k=1}^n \alpha_k \log q_k^\dag
= - \log n + \log C - \sum_{k=1}^n \alpha_k \log \alpha_k - \sum_{k=1}^n \alpha_k \log C \\
= & - \sum_{k=1}^n \alpha_k \log \alpha_k  - \log n,
\end{split}
\end{align}
where we have used the fact that $q_k^\dag = C \alpha_k$ and $\sum_{k=1}^n \alpha_k = 1$ by (\ref{eq:kkt-q}).
\item To solve (\ref{eq:L2}), by KKT conditions, $\forall j \in \tilde{V}$,
\begin{equation}
\label{eq:L2-kkt}
\frac{\partial L_2\left(\btheta^\dag\right) }{\partial \theta_{ij}^\dag} = \lambda t_j^\dag - \frac{1}{n} \sum_{k=1}^n\alpha_k \tilde{x}_j^{(k)} = 0,\quad \lvert t_j^\dag \rvert \le 1,\quad t_j^\dag\theta_{ij}^\dag = \lvert \theta_{ij}^\dag \rvert,
\end{equation}
where $t_j^\dag$ is the $j^{th}$ component of $\bt^\dag \in \partial \left(\sum_{j \in \tilde{V}} \left\lvert \theta_{ij}^\dag \right\rvert\right)$.
From (\ref{eq:L2-kkt}), we also have that
\begin{equation}
\label{eq:L2-theta-hat}
t_j^\dag = \frac{1}{n \lambda} \sum_{k=1}^n\alpha_k \tilde{x}_j^{(k)} \Rightarrow
\theta_{ij}^\dag \left(\frac{1}{n \lambda} \sum_{k=1}^n\alpha_k \tilde{x}_j^{(k)}\right) = \lvert \theta_{ij}^\dag \rvert\Rightarrow
\sum_{k=1}^n \alpha_k \tilde{x}_j^{(k)} \in
\begin{cases}
n\lambda, & \text{if } \theta_{ij}^\dag >0;\\
-n\lambda, & \text{if } \theta_{ij}^\dag <0;\\
[-n\lambda,n\lambda], & \text{if } \theta_{ij}^\dag = 0.
\end{cases}
\end{equation}

For $\theta_{ii}^\dag$, by KKT conditions, 
\begin{equation}
\label{eq:L2-theta-ii}
\sum_{k=1}^n \alpha_k x_i^{(k)}= 0.
\end{equation}
From (\ref{eq:L2-theta-hat}) and (\ref{eq:L2-theta-ii}), let $\btheta = \btheta^\dag$ in $L_2(\btheta)$. We have that
\begin{equation}
\label{eq:L2-min}
\min_{\btheta} L_2(\btheta) = L_2(\btheta^\dag) = 0.
\end{equation}

From (\ref{eq:kkt-q}), (\ref{eq:kkt-q-2}), (\ref{eq:kkt-q-3}), (\ref{eq:L2-theta-hat}), (\ref{eq:L2-theta-ii}), and (\ref{eq:L2-min}), we can conclude that the dual problem is of the form in (\ref{eq:dual}).
\end{itemize}

\subsection{Proof of Lemma~\ref{lemma:primal-dual-opt-sol}}
By strong duality given in Lemma~\ref{lemma:strong-dual}, when $\balpha = \hat{\balpha}$ in Section~\ref{sec:proof-lemma-dual}, we have that $\btheta^\dag = \hat{\btheta}$. Then by (\ref{eq:L2-theta-hat}), we can conclude that Lemma~\ref{lemma:primal-dual-opt-sol} is true.

\subsection{Proof of Lemma~\ref{lemma:lambda-max}}
\subsubsection{Determining $\hat{\theta}_{ii}$}
To decide $\hat{\theta}_{ii}$, we consider the optimality condition of interaction screening when $\hat{\btheta}_{\backslash i} = \bzero$. From (\ref{eq:primal-kkt}), 
\begin{equation}
\label{eq:primal-0-ii}
\sum_{k=1}^n \exp \left(- \hat{\theta}_{ii} x_i^{(k)} \right) x_i^{(k)} = 0 \Rightarrow \lvert \mathcal{P}_i \rvert \exp(-\hat{\theta}_{ii}) = \lvert \mathcal{N}_i \rvert \exp(\hat{\theta}_{ii})
\Rightarrow  \hat{\theta}_{ii} =  \frac{1}{2} \log \frac{ \lvert \mathcal{P}_i \rvert}{ \lvert \mathcal{N}_i \rvert}.
\end{equation}
Here, $\mathcal{P}_i := \curly{k \mid x_i^{(k)} = 1, k \in \curly{1,2,\cdots,n}}$ and  $\mathcal{N}_i := \curly{k \mid x_i^{(k)} = -1, k \in \curly{1,2,\cdots,n}}$.  $\lvert \mathcal{P}_i \rvert$ and $\lvert  \mathcal{N}_i \rvert$ represent the cardinality of $\mathcal{P}_i$ and $\mathcal{N}_i$, respectively. Note that (\ref{eq:primal-0-ii}) also dictates that $\lvert \mathcal{P}_i \rvert > 0$ and $\lvert  \mathcal{N}_i \rvert > 0$.

\subsubsection{Determining $\lambda_{\max}$}
Furthermore, when $\hat{\btheta}_{\backslash i} = \bzero$, using (\ref{eq:primal-0-ii}), we have
\begin{align}
\label{eq:partition}
\begin{split}
& \sum_{k=1}^n \exp \left(- \hat{\theta}_{ii} x_i^{(k)} \right)
= \sum_{k\in \mathcal{P}_i} \exp \left(- \hat{\theta}_{ii} x_i^{(k)} \right) + \sum_{k\in \mathcal{N}_i} \exp \left(- \hat{\theta}_{ii} x_i^{(k)} \right) = \lvert \mathcal{P}_i  \rvert \exp \left( - \hat{\theta}_{ii}  \right) + \lvert \mathcal{N}_i  \rvert \exp \left( \hat{\theta}_{ii}  \right)\\
= & \lvert \mathcal{P}_i  \rvert \exp \left( - \frac{1}{2} \log \frac{ \lvert \mathcal{P}_i \rvert}{ \lvert \mathcal{N}_i \rvert}  \right) + \lvert \mathcal{N}_i  \rvert \exp \left( \frac{1}{2} \log \frac{ \lvert \mathcal{P}_i \rvert}{ \lvert \mathcal{N}_i \rvert} \right) = 2 \sqrt{\lvert \mathcal{P}_i \rvert \lvert \mathcal{N}_i \rvert}.
\end{split}
\end{align}

From (\ref{eq:primal-kkt}), when $\hat{\btheta}_{\backslash i} = \bzero$, with (\ref{eq:primal-0-ii}) and (\ref{eq:partition}),
\begin{align}
\label{eq:primal-opt-ij}
 - & \sum_{k=1}^n \frac{ \exp \left(- \hat{\theta}_{ii} x_i^{(k)} \right) }{\sum_{k'=1}^n \exp \left(- \hat{\theta}_{ii} x_i^{(k')} \right)} \tilde{x}_{j}^{(k)} + \lambda_{\max} \hat{t}_j = 0 \nonumber \\
\Rightarrow & \sum_{k\in \mathcal{P}_i} \frac{ \exp \left(- \hat{\theta}_{ii} x_i^{(k)} \right) }{\sum_{k'=1}^n \exp \left(- \hat{\theta}_{ii} x_i^{(k')} \right)} \tilde{x}_{j}^{(k)} + \sum_{k\in \mathcal{N}_i} \frac{ \exp \left(- \hat{\theta}_{ii} x_i^{(k)} \right) }{\sum_{k'=1}^n \exp \left(- \hat{\theta}_{ii} x_i^{(k')} \right)} \tilde{x}_{j}^{(k)} = \lambda_{\max} \hat{t}_j \nonumber \\
\Rightarrow &  \sum_{k\in \mathcal{P}_i}\frac{\exp \left(- \hat{\theta}_{ii} \right) }{\sum_{k'=1}^n \exp \left(- \hat{\theta}_{ii} x_i^{(k')} \right)} x_{j}^{(k)} -   \sum_{k\in \mathcal{N}_i} \frac{ \exp \left(\hat{\theta}_{ii}  \right) }{\sum_{k'=1}^n \exp \left(- \hat{\theta}_{ii} x_i^{(k')} \right)} x_{j}^{(k)} = \lambda_{\max} \hat{t}_j \nonumber \\
\Rightarrow &  \sum_{k\in \mathcal{P}_i}\frac{\exp \left(- \frac{1}{2} \log \frac{ \lvert \mathcal{P}_i \rvert}{ \lvert \mathcal{N}_i \rvert} \right) }{2 \sqrt{\lvert \mathcal{P}_i \rvert \lvert \mathcal{N}_i \rvert}} x_{j}^{(k)} -   \sum_{k\in \mathcal{N}_i} \frac{ \exp \left( \frac{1}{2} \log \frac{ \lvert \mathcal{P}_i \rvert}{ \lvert \mathcal{N}_i \rvert}  \right) }{2 \sqrt{\lvert \mathcal{P}_i \rvert \lvert \mathcal{N}_i \rvert}} x_{j}^{(k)} = \lambda_{\max} \hat{t}_j \nonumber \\
\Rightarrow & \frac{1}{2 \lvert \mathcal{P}_i \rvert}\sum_{k\in \mathcal{P}_i} x_j^{(k)} - \frac{1}{2 \lvert \mathcal{N}_i \rvert}\sum_{k\in \mathcal{N}_i} x_j^{(k)} = \lambda_{\max} \hat{t}_j.
\end{align}
In (\ref{eq:primal-opt-ij}), by the fact that $\hat{t}_j$ is a component of the subgradient, $\lambda_{\max}$ can be determined analytically via:
\begin{equation}
\label{eq:lambda-max}
\lambda_{\max} = \max_{j\in \tilde{V}} \left\lvert \frac{1}{2 \lvert \mathcal{P}_i \rvert}\sum_{k\in \mathcal{P}_i} x_j^{(k)} - \frac{1}{2 \lvert \mathcal{N}_i \rvert}\sum_{k\in \mathcal{N}_i} x_j^{(k)} \right\rvert \le 1,
\end{equation}
where the upper bound 1 is due to the triangular inequality and the fact that $x_j^{(k)} \in \curly{-1,1}$, $\forall k \in \curly{1,\cdots,n}$, and $\forall j \in \tilde{V}$.

\subsection{Proof of Lemma~\ref{lemma:strong-dual}}
We first show that strong duality holds for given $\mathbb{X}$ and $\lambda \in (0,\lambda_{\max}]$. Since (\ref{eq:interScreen}) is convex and is equivalent to the constrained problem (\ref{eq:interScreen-eq}), we need to verify whether Slater's conditions can be satisfied for (\ref{eq:interScreen-eq}). This is trivially true. Therefore, strong duality holds. Now let $\lambda = \lambda_{\max}$. Then when $\balpha = \hat{\balpha}(\lambda_{\max})$ in Section~\ref{sec:proof-lemma-dual}, by strong duality, $\btheta^\dag = \hat{\btheta}$, with $\hat{\btheta}_{\backslash i} = \bzero$. Furthermore, by strong duality, $\btheta^\dag = \hat{\btheta}$,  (\ref{eq:interScreen-eq}), (\ref{eq:kkt-q}), the definition of $C$ in (\ref{eq:kkt-q-3}), (\ref{eq:primal-0-ii}), and (\ref{eq:partition}),
\begin{equation*}
\hat{\alpha}_k(\lambda_{\max}) = \frac{\exp \left(- \hat{\theta}_{ii} x_i^{(k)} \right)}{C} = \begin{cases}
\frac{\sqrt{\lvert \mathcal{P}_i \rvert \lvert \mathcal{N}_i \rvert}}{2\lvert \mathcal{P}_i \rvert^2} & \forall k \in \mathcal{P}_i,\\
\frac{\sqrt{\lvert \mathcal{P}_i \rvert \lvert \mathcal{N}_i \rvert}}{2\lvert \mathcal{N}_i \rvert^2} & \forall k \in \mathcal{N}_i.
\end{cases}
\end{equation*}

\subsection{Proof of Lemma~\ref{lemma:strong-cvx}}
In (\ref{eq:grad-hessian}), the expression of the gradient and hessian can be obtained trivially by differentiation. Furthermore, $\balpha\in \mathcal{B} \Rightarrow \nabla^2 g(\balpha) \ge \frac{1}{n}\mathbf{I}$, where $\mathbf{I}$ is the identity matrix. Therefore, $g (\balpha)$ is strongly convex in $\mathcal{B}$ with modulus $\frac{1}{n}$, yielding the inequality (\ref{eq:ball}).

\subsection{Proof of Lemma~\ref{lemma:dual-kkt}}
The dual problem (\ref{eq:dual}) can be rewritten as:
\begin{align}
\hat{\balpha} = \arg\min_{\balpha}\ & g(\balpha),\nonumber \\
\label{eq:dual-con-1}
\text{s.t.\quad} & \sum_{k=1}^n \alpha_k  \tilde{x}_j^{(k)} - n\lambda \le 0,\quad \forall j \in \tilde{V},\\
\label{eq:dual-con-2}
 -& \sum_{k=1}^n \alpha_k \tilde{x}_j^{(k)} - n\lambda \le 0,\quad \forall j \in \tilde{V},\\
 \label{eq:dual-con-5}
& \sum_{k=1}^n \alpha_k x_i^{(k)} = 0,\\
\label{eq:dual-con-3}
& \sum_{k=1}^n \alpha_k - 1 =0,\\
\label{eq:dual-con-4}
& \balpha \in \mathcal{B},
\end{align}
where $g(\balpha)$ and $\mathcal{B}$ are defined in Lemma~\ref{lemma:strong-cvx}. At optimality,
\begin{equation}
\label{eq:dual-kkt}
\bzero \in \nabla g\left(\hat{\balpha}\right) + \sum_{j \in \tilde{V}} \gamma^+_j \tilde{\bx}_j - \sum_{j \in \tilde{V}} \gamma^-_j \tilde{\bx}_j + \kappa_1 \bx_i + \kappa_2 \bone + N_\mathcal{B}\left(\hat{\balpha}\right),
\end{equation}
where $\gamma^+_j\ge 0$, $\forall j \in \tilde{V}$, are the slack variables corresponding to the constraints in (\ref{eq:dual-con-1}); $\gamma^-_j \ge 0$, $\forall j \in \tilde{V}$, are the slack variables corresponding to the constraints in (\ref{eq:dual-con-2}); $\kappa_1 \in \mathbb{R}$ is the slack variable corresponding to the constraint in (\ref{eq:dual-con-5}); $\kappa_2 \in \mathbb{R}$ is the slack variable corresponding to the constraint in (\ref{eq:dual-con-3}); $\bx_i = \begin{bmatrix} x_i^{(1)} & x_i^{(2)} & \cdots & x_i^{(n)} \end{bmatrix}^\top$;  $\bone$ is an $n\times 1$ vector of all ones; $N_\mathcal{B}\left(\hat{\balpha}\right)$ is the normal cone of the set $\mathcal{B}$ in (\ref{eq:dual-con-4}) at $\hat{\balpha}$. Note that $\mathcal{B}$ is an open set and $\hat{\balpha} \in \mathcal{B}$ is an interior point of $\mathcal{B}$. We have that $N_{\mathcal{B}}\left(\hat{\balpha}\right) = \curly{\bzero}$. Therefore, (\ref{eq:dual-kkt}) can be further simplified as
\begin{equation*}
\nabla g \left(\hat{\balpha}\right) + \sum_{j \in \tilde{V}} \gamma^+_j \tilde{\bx}_j - \sum_{j \in \tilde{V}} \gamma^-_j \tilde{\bx}_j + \kappa_1 \bx_i + \kappa_2 \bone = \bzero.
\end{equation*}

\subsection{Further Refining $\mathcal{R}(\lambda)$}
From (\ref{eq:dual-con-5}), we have that $\hat{\balpha}(\lambda)^\top \bx_i = \hat{\balpha}(\lambda_0)^\top \bx_i = 0$. Therefore, $\left(\hat{\balpha}(\lambda) - \hat{\balpha}(\lambda_0)\right)^\top \bx_i = 0$.
Similarly, from (\ref{eq:dual-con-3}), we have that $\hat{\balpha}(\lambda)^\top \bone = \hat{\balpha}(\lambda_0)^\top \bone = 1$. Therefore, $\left(\hat{\balpha}(\lambda) - \hat{\balpha}(\lambda_0)\right)^\top \bone = 0$. Therefore, we can conclude that  $\left(\hat{\balpha}(\lambda) - \hat{\balpha}(\lambda_0)\right)$ is in the nullspace of $\mathbf{S}:=\begin{bmatrix} \bx_i & \bone \end{bmatrix}^\top$.

On the other hand, by (\ref{eq:U_j}),
\small
\begin{equation}
\label{eq:screen-3}
U_j(\lambda) = \max \curly{\left[\max_{\balpha\in\mathcal{R}(\lambda)} \left(\balpha - \hat{\balpha}(\lambda_0)\right)^\top \tilde{\bx}_j\right]+\hat{\balpha}(\lambda_0)^\top \tilde{\bx}_j,\ \left[\max_{\balpha\in\mathcal{R}(\lambda)} \left(\balpha - \hat{\balpha}(\lambda_0)\right)^\top \left(-\tilde{\bx}_j\right)\right] - \hat{\balpha}(\lambda_0)^\top \tilde{\bx}_j}.
\end{equation}
\normalsize
Let $\mathcal{R}(\lambda) := \curly{\balpha \mid \norm{\balpha - \hat{\balpha}(\lambda_0)}_2 \le r,\ \mathbf{S} \left(\balpha-\hat{\balpha}(\lambda_0)\right) = 0,\ \bk^\top \left(\balpha-\hat{\balpha}(\lambda_0)\right) \le b}$, where $\bk$ is an $n\times 1$ data vector that depends on $\mathbb{X}$, and $b$ is a constant. In this way, we consider a region $\mathcal{R}(\lambda)$ that is constructed by the two equality constraints in the dual problem (\ref{eq:dual}), the ball constraint given in (\ref{eq:ball}), and potentially one of the half space constraints given in the dual problem via (\ref{eq:dual-con-2}) and (\ref{eq:dual-con-3}).

Let $\bmeta = \balpha - \hat{\balpha}(\lambda_0)$. To solve (\ref{eq:screen-3}), without loss of generality, we can first consider the following optimization problem:
\begin{subequations}
\label{eq:u-plus}
\begin{align}
-U_+:=\min_{\bmeta}\quad & \bmeta^\top (-\tilde{\bx}_j), \\
\label{eq:u-plus-b}
\text{s.t.}\quad & \norm{\bmeta}_2^2 \le r^2,\\
\label{eq:u-plus-c}
& \bk^\top \bmeta \le b,\\
\label{eq:u-plus-d}
& \bx_i^\top \bmeta = 0,\\
\label{eq:u-plus-e}
& \bm{1}^\top \bmeta = 0,\\
\label{eq:u-plus-f}
- & \be_k^\top \bmeta \le \hat{\alpha}_k(\lambda_0),\quad k \in \clC \subseteq \curly{1,2,\cdots,n}.
\end{align}
\end{subequations}

To solve (\ref{eq:u-plus}), we will adopt the Lagrange multiplier method \charles{Technically, we need to check that strong duality holds}. To proceed, we first write down the Lagrangian of (\ref{eq:u-plus}):
\begin{align}
\label{eq:u-plus-lag}
\mathcal{L}(\bmeta; u_1, u_2, v_1, v_2, \bmu) & = \check{\bx}_j^\top \bmeta + \frac{u_1}{2} \left(\norm{\bmeta}_2^2-r^2\right) + u_2 \left(\bk^\top \bmeta - b\right) - \sum_{k \in \clC} \mu_k \left( \be_k^\top \bmeta +\hat{\alpha}_k(\lambda_0) \right) + v_1 \left(\bx_i^\top \bmeta\right) + v_2 \left(\bone^\top \bmeta\right)\nonumber \\
& = \left(\check{\bx}_j + u_2 \bk - \sum_{k \in \clC} \mu_k \be_k + v_1 \bx_i + v_2 \bone\right)^\top \bmeta + \frac{u_1}{2} \left(\norm{\bmeta}_2^2-r^2\right) - u_2 b - \sum_{k \in \clC} \mu_k \hat{\alpha}_k(\lambda_0),
\end{align}
where $u_1\ge0$, $u_2\ge0$, and $\bmu \ge \bzero$ are the Lagrange multipliers corresponding to the constraints (\ref{eq:u-plus-b}), (\ref{eq:u-plus-c}), and (\ref{eq:u-plus-f}); and $v_1\in \mathbb{R}$ and $v_2\in \mathbb{R}$ are the Lagrange multipliers corresponding to the constraints (\ref{eq:u-plus-d}) and (\ref{eq:u-plus-e}). Moreover, $\check{\bx}_j = -\tilde{\bx}_j$. Let $\nabla_{\bmeta} \mathcal{L}(\bmeta; u_1, u_2, v_1, v_2, \bmu) = 0$. We have that
\begin{equation*}
\check{\bx}_j + u_2 \bk - \sum_{k \in \clC} \mu_k \be_k + v_1 \bx_i + v_2 \bone + u_1 \bmeta = \bzero.
\end{equation*}
When $u_1 \ne 0$, we have that
\begin{equation}
\label{eq:u-plus-lag-opt-1}
\bmeta = -\frac{1}{u_1} \left(\check{\bx}_j + u_2 \bk - \sum_{k \in \clC} \mu_k \be_k + v_1 \bx_i + v_2 \bone\right).
\end{equation}
Plugging (\ref{eq:u-plus-lag-opt-1}) into (\ref{eq:u-plus-lag}) yields the dual function:
\begin{equation*}
D(u_1, u_2, v_1, v_2, \bmu) = -\frac{1}{2u_1} \Norm{\check{\bx}_j + u_2 \bk - \sum_{k \in \clC} \mu_k \be_k  + v_1 \bx_i + v_2 \bone}_2^2 -\frac{1}{2} u_1r^2 - u_2 b - \sum_{k \in \clC} \mu_k \hat{\alpha}_k(\lambda_0).
\end{equation*}

When $u_1=0$,
\begin{equation}
\label{eq:u-plus-lag-2}
\mathcal{L}(\bmeta; u_1, u_2, v_1, v_2, \bmu) =\left(\check{\bx}_j + u_2 \bk - \sum_{k \in \clC} \mu_k \be_k + v_1 \bx_i + v_2 \bone\right)^\top \bmeta - u_2 b - \sum_{k \in \clC} \mu_k \hat{\alpha}_k(\lambda_0).
\end{equation}

In this case, when $\frac{(\bPi \check{\bx}_j)^\top \bPi \bk}{\norm{\bPi \check{\bx}_j}_2 \norm{\bPi \bk}_2} \in (-1,1]$, we would like to show that $\check{\bx}_j + u_2 \bk - \sum_{k \in \clC} \mu_k \be_k + v_1 \bx_i + v_2 \bone \ne \bzero$. Suppose otherwise, i.e.~$\exists u_2'>0$, $\mu_k'\ge 0$, $\forall k \in\clC$, $v_1'$, and $v_2'$, s.t. \charles{worry about $\norm{\bPi \check{\bx}_j}_2=\norm{\bPi \bk}_2=0$}
\begin{equation}
\label{eq:u'-1}
\check{\bx}_j + u_2' \bk - \sum_{k \in \clC} \mu_k' \be_k + v_1' \bx_i + v_2' \bone = \bzero \Rightarrow \bPi \check{\bx}_j + u_2' \bPi \bk = \bzero \Rightarrow u_2' = -\frac{(\bPi \check{\bx}_j)^\top \bPi \bk}{\norm{\bPi \bk}_2^2}.
\end{equation}
where the second equality is due to the fact that $\bPi \be_k =\bzero$, $\forall k \in \clC$; $\bPi \bx_i = \bPi \bone = \bzero$. The second equality in (\ref{eq:u'-1}) also suggests that $\bPi \check{\bx}_j$ and $\bPi \bk $ are colinear, which means $\frac{(\bPi \check{\bx}_j)^\top \bPi \bk}{\norm{\bPi \check{\bx}_j}_2 \norm{\bPi \bk}_2} \in \curly{-1,1}$. From the third equality in  (\ref{eq:u'-1}), $(\bPi \check{\bx}_j)^\top \bPi \bk \le 0$. Therefore, $\frac{(\bPi \check{\bx}_j)^\top \bPi \bk}{\norm{\bPi \check{\bx}_j}_2 \norm{\bPi \bk}_2} = -1$, which contradicts to the assumption that $\frac{(\bPi \check{\bx}_j)^\top \bPi \bk}{\norm{\bPi \check{\bx}_j}_2 \norm{\bPi \bk}_2} \in (-1,1]$.

Therefore, when  $\frac{(\bPi \check{\bx}_j)^\top \bPi \bk}{\norm{\bPi \check{\bx}_j}_2 \norm{\bPi \bk}_2} \in (-1,1]$, $\check{\bx}_j + u_2 \bk - \sum_{k \in \clC} \mu_k \be_k + v_1 \bx_i + v_2 \bone \ne \bzero$. In this case, (\ref{eq:u-plus-lag-2}) is linear with respect to $\bmeta$, and hence $\min_{\bmeta} \mathcal{L}(\bmeta; u_1, u_2, v_1, v_2, \bmu)=-\infty$.

To sum up, when $\frac{(\bPi \check{\bx}_j)^\top \bPi \bk}{\norm{\bPi \check{\bx}_j}_2 \norm{\bPi \bk}_2} \in (-1,1]$, the dual problem is:
\begin{equation}
\label{eq:u-plus-dual}
\max_{u_1>0,u_2\ge0,v_1,v_2,\bmu\ge0} -\frac{1}{2u_1} \Norm{-\check{\bx}_j - u_2 \bk + \sum_{k \in \clC} \mu_k \be_k  - \begin{bmatrix} \bone & \bx_i\end{bmatrix} \begin{bmatrix}
v_2 \\ v_1
\end{bmatrix}}_2^2 -\frac{1}{2} u_1r^2 - u_2 b - \sum_{k \in \clC} \mu_k \hat{\alpha}_k(\lambda_0).
\end{equation}
The optimization with respect to $v_1$ and $v_2$ can be viewed as a simple linear regression problem, where
\begin{subequations}
\label{eq:opt-v1-v2}
\begin{align}
\hat{v}_1 = & \frac{\text{Cov}\left(\bx_i,-\check{\bx}_j - u_2 \bk + \sum_{k \in \clC} \mu_k \be_k\right)}{\text{Var}(\bx_i)} 
= -\frac{\text{Cov}(\bx_i,\check{\bx}_j)}{\text{Var}(\bx_i)} - u_2\frac{\text{Cov}(\bx_i,\bk)}{\text{Var}(\bx_i)} + \sum_{k\in\clC} \mu_k \frac{\text{Cov}(\bx_i,\be_k)}{\text{Var}(\bx_i)}\\
\hat{v}_2 = & -\mathbb{E} \check{\bx}_j - u_2 \mathbb{E} \bk + \sum_{k\in\clC}\frac{\mu_k}{n} - \hat{v}_1 \mathbb{E}\bx_i\nonumber \\
= & \left(\frac{\text{Cov}(\bx_i,\bk)}{\text{Var}(\bx_i)}\mathbb{E}\bx_i -\mathbb{E} \bk \right)  u_2 + \sum_{k\in\clC} \left(\frac{1}{n}-\frac{\text{Cov}(\bx_i,\be_k)}{\text{Var}(\bx_i)}\mathbb{E}\bx_i\right) \mu_k -  \mathbb{E} \check{\bx}_j + \frac{\text{Cov}(\bx_i,\check{\bx}_j)}{\text{Var}(\bx_i)}\mathbb{E}\bx_i.
\end{align}
\end{subequations}
Plug (\ref{eq:opt-v1-v2}) into (\ref{eq:u-plus-dual}) yields:
\begin{align}
\label{eq:u-plus-dual-2}
\begin{split}
\max_{u_1>0,u_2\ge0,\bmu\ge0} & -\frac{1}{2u_1} \Norm{\left[-\bk -\left(\frac{\text{Cov}(\bx_i,\bk)}{\text{Var}(\bx_i)}\mathbb{E}\bx_i - \mathbb{E} \bk\right) \bone + \frac{\text{Cov}(\bx_i,\bk)}{\text{Var}(\bx_i)} \bx_i \right]u_2 \right. \\ 
& \left.
+ \sum_{k\in\clC} \left[ \be_k -\left(\frac{1}{n}-\frac{\text{Cov}(\bx_i,\be_k)}{\text{Var}(\bx_i)}\mathbb{E}\bx_i\right) \bone - \frac{\text{Cov}(\bx_i,\be_k)}{\text{Var}(\bx_i)} \bx_i  \right] \mu_k 
 \right. \\ 
& \left.
- \check{\bx}_j + \left(\mathbb{E} \check{\bx}_j - \frac{\text{Cov}(\bx_i,\check{\bx}_j)}{\text{Var}(\bx_i)}\mathbb{E}\bx_i\right)\bone +
 \frac{\text{Cov}(\bx_i,\check{\bx}_j)}{\text{Var}(\bx_i)} \bx_i
}_2^2 \\
& -\frac{1}{2} u_1r^2 - u_2 b - \sum_{k \in \clC} \mu_k \hat{\alpha}_k(\lambda_0).
\end{split}
\end{align}

Other other hand, when $\frac{(\bPi \check{\bx}_j)^\top \bPi \bk}{\norm{\bPi \check{\bx}_j}_2 \norm{\bPi \bk}_2} =-1$,
\begin{equation}
\label{eq:u'-1}
\check{\bx}_j + u_2 \bk - \sum_{k \in \clC} \mu_k \be_k + v_1 \bx_i + v_2 \bone = \bzero \Rightarrow  u_2 = -\frac{(\bPi \check{\bx}_j)^\top \bPi \bk}{\norm{\bPi \bk}_2^2}.
\end{equation}
\charles{the dual problem here is incomplete}

Let
\begin{align*}
& \ba := -\bk -\left(\frac{\text{Cov}(\bx_i,\bk)}{\text{Var}(\bx_i)}\mathbb{E}\bx_i - \mathbb{E} \bk\right) \bone + \frac{\text{Cov}(\bx_i,\bk)}{\text{Var}(\bx_i)} \bx_i, \\
& \bb_k := \be_k -\left(\frac{1}{n}-\frac{\text{Cov}(\bx_i,\be_k)}{\text{Var}(\bx_i)}\mathbb{E}\bx_i\right) \bone - \frac{\text{Cov}(\bx_i,\be_k)}{\text{Var}(\bx_i)} \bx_i,\\
& \bc := - \check{\bx}_j + \left(\mathbb{E} \check{\bx}_j - \frac{\text{Cov}(\bx_i,\check{\bx}_j)}{\text{Var}(\bx_i)}\mathbb{E}\bx_i\right)\bone +
 \frac{\text{Cov}(\bx_i,\check{\bx}_j)}{\text{Var}(\bx_i)} \bx_i.
\end{align*}

Consider
\begin{equation*}
\min_{u_1>0,u_2\ge0,\bmu\ge0} \frac{1}{2u_1}\Norm{\ba u_2 + \sum_{k\in\clC} \bb_k \mu_k + \bc}_2^2 +\frac{1}{2} u_1r^2 +  u_2 b +  \sum_{k \in \clC}  \mu_k \hat{\alpha}_k(\lambda_0).
\end{equation*}

Introducing slack variables, at optimality,
\begin{align*}
-\frac{1}{2u_1^2}\Norm{\ba u_2 + \sum_{k'\in\clC} \bb_{k'} \mu_{k'} + \bc}_2^2 + \frac{1}{2}r^2 - s_1 & = 0,\\
\frac{1}{u_1}\ba^\top \left(\ba u_2 + \sum_{k'\in\clC} \bb_{k'} \mu_{k'} + \bc\right) + b - s_2 & = 0,\\
\frac{1}{u_1}\bb_k^\top \left(\ba u_2 + \sum_{k'\in\clC} \bb_{k'} \mu_{k'} + \bc\right) + \hat{\alpha}_k(\lambda_0) - t_k& = 0,\quad \forall k \in \clC, \\
s_1 u_1 =0,\quad s_2 u_2 =0,\quad t_k \mu_k &= 0,\quad \forall k \in \clC.
\end{align*}
At optimality, since $u_1>0$, $s_1=0$, therefore,
\begin{gather*}
u_1 = \frac{\Norm{\ba u_2 + \sum_{k\in\clC} \bb_k \mu_k + \bc}_2}{r},\\
\frac{\ba^\top \left(\ba u_2 + \sum_{k'\in\clC} \bb_{k'} \mu_{k'} + \bc\right)}{\Norm{\ba u_2 + \sum_{k\in\clC} \bb_k \mu_k + \bc}_2 \norm{\ba}_2} = \frac{s_2-b}{r \norm{\ba}_2},\quad 
\frac{\bb_k^\top \left(\ba u_2 + \sum_{k'\in\clC} \bb_{k'} \mu_{k'} + \bc\right) }{\Norm{\ba u_2 + \sum_{k\in\clC} \bb_k \mu_k + \bc}_2\norm{\bb_k}_2} = \frac{t_k - \hat{\alpha}_k(\lambda_0)}{r \norm{\bb_k}_2}.
\end{gather*}
When it is $\mu$ free,
\begin{equation*}
u_1 = \frac{\Norm{\ba u_2 + \bc}_2}{r}, \quad \frac{\ba^\top \left(\ba u_2 + \bc\right)}{\Norm{\ba u_2 + \bc}_2 \norm{\ba}_2} = \frac{s_2-b}{r \norm{\ba}_2} \ge \frac{\ba^\top \bc}{\norm{\ba}_2\norm{\bc}_2}.
\end{equation*}
If we further assume that $-\frac{b}{r \norm{\ba}_2} > \frac{\ba^\top \bc}{\norm{\ba}_2\norm{\bc}_2}$, then $s_2>0$, and hence $u_2=0$. If $-\frac{b}{r \norm{\ba}_2} = \frac{\ba^\top \bc}{\norm{\ba}_2\norm{\bc}_2}$, and we further assume that $u_2>0$, $s_2=0$ by complementary slackness. In this case, $ \frac{\ba^\top \left(\ba u_2 + \bc\right)}{\Norm{\ba u_2 + \bc}_2 \norm{\ba}_2} = -\frac{b}{r \norm{\ba}_2} $ is a constant $\forall u_2>0$, which is not true. When $-\frac{b}{r \norm{\ba}_2} = \frac{\ba^\top \bc}{\norm{\ba}_2\norm{\bc}_2}$, $u_2=0$ must be true.

On the other hand, when $-\frac{b}{r \norm{\ba}_2} < \frac{\ba^\top \bc}{\norm{\ba}_2\norm{\bc}_2}$, if $u_2 =0$, then
\begin{equation*}
\frac{\ba^\top \left(\ba u_2 + \bc\right)}{\Norm{\ba u_2 + \bc}_2 \norm{\ba}_2} = \frac{\ba^\top \bc}{\norm{\ba}_2\norm{\bc}_2},\quad \frac{\ba^\top \left(\ba u_2 + \bc\right)}{\Norm{\ba u_2 + \bc}_2 \norm{\ba}_2}=\frac{s_2-b}{r \norm{\ba}_2} \Rightarrow s_2 <0,
\end{equation*}
which is a contradiction. Therefore, when $-\frac{b}{r \norm{\ba}_2} < \frac{\ba^\top \bc}{\norm{\ba}_2\norm{\bc}_2}$, $u_2>0$ must be true and hence by complementary slackness, $s_2=0$.  \charles{not finished yet}
